# Supplementary material for: Legged Robot State-Estimation Through Combined Forward Kinematic and Preintegrated Contact Factors
Source: arXiv:1712.05873 ancillary file (2018-02-25)
Supplement: Supplementary file 1 [file icra-supplementary-material.pdf]

# Supplementary Material to: Legged Robot State-Estimation Through Combined Kinematic and Preintegrated Contact Factors

Ross Hartley, Josh Mangelson, Lu Gan, Maani Ghaffari Jadidi, Jeffrey M. Walls,  
Ryan M. Eustice, and Jessy W. Grizzle

February 25, 2018

This technical report provides detailed derivations of the of the equations presented in [1]. It is not self-contained and therefore should be read alongside the main paper. Where possible, we adopt the styling and notion conventions of [2], as this work can be viewed as an extension of IMU preintegration theory. References in **red** refer to equations in the main paper [1].

## Contents

|          |                                                              |           |
|----------|--------------------------------------------------------------|-----------|
| <b>1</b> | <b>Forward Kinematic Factor Derivations</b>                  | <b>2</b>  |
| 1.1      | Factorization of Joint Offsets . . . . .                     | 2         |
| 1.2      | Measurement Model . . . . .                                  | 2         |
| 1.3      | Residuals and Covariance . . . . .                           | 5         |
| <b>2</b> | <b>Forward Kinematic Factor Jacobians</b>                    | <b>6</b>  |
| 2.1      | Jacobians of $\mathbf{r}_{f_R}$ . . . . .                    | 6         |
| 2.2      | Jacobians of $\mathbf{r}_{f_p}$ . . . . .                    | 7         |
| <b>3</b> | <b>Rigid Contact Factor Derivations</b>                      | <b>7</b>  |
| 3.1      | Measurement Model . . . . .                                  | 7         |
| 3.2      | Residuals and Covariance . . . . .                           | 9         |
| <b>4</b> | <b>Rigid Contact Factor Jacobians</b>                        | <b>9</b>  |
| 4.1      | Jacobians of $\mathbf{r}_{\Delta \mathbf{C}_{ij}}$ . . . . . | 9         |
| 4.2      | Jacobians of $\mathbf{r}_{\Delta \mathbf{d}_{ij}}$ . . . . . | 10        |
| <b>5</b> | <b>Point Contact Factor Derivations</b>                      | <b>11</b> |
| 5.1      | Measurement Model . . . . .                                  | 11        |
| 5.2      | Iterative Noise Propagation . . . . .                        | 12        |
| 5.3      | Separation of IMU and Contact Factors . . . . .              | 13        |
| <b>6</b> | <b>Point Contact Factor Jacobians</b>                        | <b>13</b> |
| 6.1      | Jacobians of $\mathbf{r}_{\Delta \mathbf{d}_{ij}}$ . . . . . | 13        |

# 1 Forward Kinematic Factor Derivations

## 1.1 Factorization of Joint Offsets

**Lemma 1** (Relative rotation between two frames). *Let  $\beta \in \mathbb{R}^N$  be a vector of joint angle offsets. The relative rotation between frames  $i$  and  $j$  can be factored into the nominal rotation and an offset rotation:*

$$\mathbf{A}_{ij}(\alpha + \beta) = \mathbf{A}_{ij}(\alpha) \prod_{k=i}^{j-1} \text{Exp} \left( \mathbf{A}_{k+1,j}^\top(\alpha) \beta_k^\dagger \right) \quad (1)$$

*Proof.* Successive rotations about the same axis commute, therefore for any particular joint:

$$\text{Exp}((\alpha_n + \beta_n)^\dagger) = \text{Exp}(\alpha_n^\dagger) \text{Exp}(\beta_n^\dagger) \quad (2)$$

This property together with adjoint representation of  $\text{SO}(3)$  allow the relative rotation between frames  $i$  and  $j$  can be factored into the nominal rotation and an offset rotation:

$$\begin{aligned} \mathbf{A}_{ij}(\alpha + \beta) &= \prod_{k=i}^{j-1} \mathbf{A}_k \text{Exp}((\alpha_k + \beta_k)^\dagger) \\ &= \prod_{k=i}^{j-1} \mathbf{A}_k \text{Exp}(\alpha_k^\dagger) \text{Exp}(\beta_k^\dagger) \\ &\stackrel{\text{eq.(3)}}{=} \mathbf{A}_{ij}(\alpha) \prod_{k=i}^{j-1} \text{Exp} \left( \mathbf{A}_{k+1,j}^\top(\alpha) \beta_k^\dagger \right) \end{aligned} \quad (3)$$

□

## 1.2 Measurement Model

This section provides the complete derivations behind the forward kinematic factor equations presented in Section IV. Starting with (16), we can write the forward kinematics equations at time  $t$  as:

$$\begin{aligned} \mathbf{R}^\top \mathbf{C} &= \mathbf{f}_R(\tilde{\alpha} - \eta^\alpha) \\ \mathbf{R}^\top (\mathbf{d} - \mathbf{p}) &= \mathbf{f}_p(\tilde{\alpha} - \eta^\alpha) \end{aligned} \quad (4)$$

In order to create a factor from these measurements, we need to isolate the noise terms.

**Lemma 2** (FK factor orientation noise isolation). *Using (12), (13), and (3), the rotation term and the noise quantity  $\delta \mathbf{f}_R$  can be derived as*

$$\begin{aligned} \mathbf{R}^\top \mathbf{C} &= \mathbf{f}_R(\tilde{\alpha} - \eta^\alpha) \\ &= \mathbf{f}_R(\tilde{\alpha}) \prod_{k=1}^{N-1} \text{Exp} \left( -\mathbf{A}_{k+1,N+1}^\top(\tilde{\alpha}) \eta_k^{\alpha^\dagger} \right) \triangleq \mathbf{f}_R(\tilde{\alpha}) \text{Exp}(-\delta \mathbf{f}_R) \end{aligned} \quad (5)$$

$$\begin{aligned} \delta \mathbf{f}_R &= -\text{Log} \left( \prod_{k=1}^{N-1} \text{Exp} \left( -\mathbf{A}_{k+1,N+1}^\top(\tilde{\alpha}) \eta_k^{\alpha^\dagger} \right) \right) \\ &\approx \sum_{k=1}^{N-1} \mathbf{A}_{k+1,N+1}^\top(\tilde{\alpha}) \eta_k^{\alpha^\dagger} \end{aligned} \quad (6)$$

Through repeated first order approximation, the noise quantity  $\delta \mathbf{f}_R$  is approximately zero mean and Gaussian.

*Proof.*

$$\begin{aligned} \mathbf{R}^\top \mathbf{C} &= \mathbf{f}_R(\tilde{\alpha} - \eta^\alpha) \\ &\stackrel{\text{eq.(12)}}{=} \mathbf{A}_{1N}(\tilde{\alpha} - \eta^\alpha) \mathbf{A}_N \\ &\stackrel{\text{eq.(13)}}{=} \mathbf{A}_{1N}(\tilde{\alpha}) \left[ \prod_{k=1}^{N-1} \text{Exp} \left( -\mathbf{A}_{k+1,N}^\top(\tilde{\alpha}) \eta_k^{\alpha^\dagger} \right) \right] \mathbf{A}_N \end{aligned} \quad (7)$$

Once the product is expanded out, the adjoint property, (3), can be repeatedly used to move  $\mathbf{A}_N$  left:

$$\begin{aligned}
\mathbf{R}^\top \mathbf{C} &= \mathbf{A}_{1N}(\tilde{\alpha}) \left[ \text{Exp} \left( -\mathbf{A}_{2,N}^\top(\tilde{\alpha}) \boldsymbol{\eta}_1^{\alpha^\dagger} \right) \cdots \text{Exp} \left( -\mathbf{A}_{N-1,N}^\top(\tilde{\alpha}) \boldsymbol{\eta}_{N-2}^{\alpha^\dagger} \right) \text{Exp} \left( -\mathbf{A}_{N,N}^\top(\tilde{\alpha}) \boldsymbol{\eta}_{N-1}^{\alpha^\dagger} \right) \right] \mathbf{A}_N \\
&\stackrel{\text{eq. (3)}}{=} \mathbf{A}_{1N}(\tilde{\alpha}) \left[ \text{Exp} \left( -\mathbf{A}_{2,N}^\top(\tilde{\alpha}) \boldsymbol{\eta}_1^{\alpha^\dagger} \right) \cdots \text{Exp} \left( -\mathbf{A}_{N-1,N}^\top(\tilde{\alpha}) \boldsymbol{\eta}_{N-2}^{\alpha^\dagger} \right) \mathbf{A}_N \text{Exp} \left( -\mathbf{A}_N^\top \mathbf{A}_{N,N}^\top(\tilde{\alpha}) \boldsymbol{\eta}_{N-1}^{\alpha^\dagger} \right) \right] \\
&\stackrel{\text{eq. (3)}}{=} \mathbf{A}_{1N}(\tilde{\alpha}) \left[ \text{Exp} \left( -\mathbf{A}_{2,N}^\top(\tilde{\alpha}) \boldsymbol{\eta}_1^{\alpha^\dagger} \right) \cdots \mathbf{A}_N \text{Exp} \left( -\mathbf{A}_N^\top \mathbf{A}_{N-1,N}^\top(\tilde{\alpha}) \boldsymbol{\eta}_{N-2}^{\alpha^\dagger} \right) \text{Exp} \left( -\mathbf{A}_N^\top \mathbf{A}_{N,N}^\top(\tilde{\alpha}) \boldsymbol{\eta}_{N-1}^{\alpha^\dagger} \right) \right] \\
&\quad \vdots \\
&\stackrel{\text{eq. (3)}}{=} \mathbf{A}_{1N}(\tilde{\alpha}) \mathbf{A}_N \prod_{k=1}^{N-1} \text{Exp} \left( -\mathbf{A}_N^\top \mathbf{A}_{k+1,N}^\top(\tilde{\alpha}) \boldsymbol{\eta}_k^{\alpha^\dagger} \right) \\
&= \mathbf{f}_R(\tilde{\alpha}) \prod_{k=1}^{N-1} \text{Exp} \left( -\mathbf{A}_{k+1,N+1}^\top(\tilde{\alpha}) \boldsymbol{\eta}_k^{\alpha^\dagger} \right) \\
&\triangleq \mathbf{f}_R(\tilde{\alpha}) \text{Exp}(-\delta \mathbf{f}_R)
\end{aligned} \tag{8}$$

The noise quantity  $\delta \mathbf{f}_R$  can be shown to be approximately zero mean and Gaussian through repeated first order approximation (noting that for small rotations, the right Jacobian is close to the identity):

$$\begin{aligned}
\delta \mathbf{f}_R &= -\text{Log} \left( \prod_{k=1}^{N-1} \text{Exp} \left( -\mathbf{A}_{k+1,N+1}^\top(\tilde{\alpha}) \boldsymbol{\eta}_k^{\alpha^\dagger} \right) \right) \\
&= -\text{Log} \left( \prod_{k=1}^{N-2} \left[ \text{Exp} \left( -\mathbf{A}_{k+1,N+1}^\top(\tilde{\alpha}) \boldsymbol{\eta}_k^{\alpha^\dagger} \right) \right] \text{Exp} \left( -\mathbf{A}_{N,N+1}^\top(\tilde{\alpha}) \boldsymbol{\eta}_{N-1}^{\alpha^\dagger} \right) \right) \\
&= -\text{Log} \left( \text{Exp} \left( \text{Log} \left( \prod_{k=1}^{N-2} \text{Exp} \left( -\mathbf{A}_{k+1,N+1}^\top(\tilde{\alpha}) \boldsymbol{\eta}_k^{\alpha^\dagger} \right) \right) \right) \text{Exp} \left( -\mathbf{A}_{N,N+1}^\top(\tilde{\alpha}) \boldsymbol{\eta}_{N-1}^{\alpha^\dagger} \right) \right) \\
&\stackrel{\text{eq. (2)}}{\approx} -\text{Log} \left( \prod_{k=1}^{N-2} \text{Exp} \left( -\mathbf{A}_{k+1,N+1}^\top(\tilde{\alpha}) \boldsymbol{\eta}_k^{\alpha^\dagger} \right) \right) \\
&\quad - \mathbf{J}_r^{-1} \left( \text{Log} \left( \prod_{k=1}^{N-2} \text{Exp} \left( -\mathbf{A}_{k+1,N+1}^\top(\tilde{\alpha}) \boldsymbol{\eta}_k^{\alpha^\dagger} \right) \right) \right) \left( -\mathbf{A}_{N,N+1}^\top(\tilde{\alpha}) \boldsymbol{\eta}_{N-1}^{\alpha^\dagger} \right) \\
&\approx -\text{Log} \left( \prod_{k=1}^{N-2} \text{Exp} \left( -\mathbf{A}_{k+1,N+1}^\top(\tilde{\alpha}) \boldsymbol{\eta}_k^{\alpha^\dagger} \right) \right) + \mathbf{A}_{N,N+1}^\top(\tilde{\alpha}) \boldsymbol{\eta}_{N-1}^{\alpha^\dagger} \\
&\quad \vdots \\
&\approx \sum_{k=1}^{N-1} \mathbf{A}_{k+1,N+1}^\top(\tilde{\alpha}) \boldsymbol{\eta}_k^{\alpha^\dagger}
\end{aligned} \tag{9}$$

□

**Lemma 3** (FK factor position noise isolation). *Using (12), (13), the first order approximation of the exponential map, and anticommutativity of skew-symmetric matrices, the position term can be approximated as:*

$$\begin{aligned}
\mathbf{R}^\top (\mathbf{d} - \mathbf{p}) &= \mathbf{f}_p(\tilde{\alpha} - \boldsymbol{\eta}^\alpha) \\
&\approx \mathbf{f}_p(\tilde{\alpha}) + \sum_{k=1}^{N-1} \sum_{n=k}^{N-1} \mathbf{A}_{1,n+1}(\tilde{\alpha}) \mathbf{t}_{n+1}^\wedge \mathbf{A}_{k+1,n+1}^\top(\tilde{\alpha}) \boldsymbol{\eta}_k^{\alpha^\dagger} \\
&\triangleq \mathbf{f}_p(\tilde{\alpha}) - \delta \mathbf{f}_p
\end{aligned} \tag{10}$$

The noise quantity  $\delta \mathbf{f}_p$  is a linear combination of zero mean Gaussians, and is therefore also zero mean and Gaussian.

*Proof.*

$$\begin{aligned}
\mathbf{R}^\top(\mathbf{d} - \mathbf{p}) &= \mathbf{f}_p(\tilde{\boldsymbol{\alpha}} - \boldsymbol{\eta}^\alpha) \\
&\stackrel{\text{eq. (12)}}{=} \sum_{n=1}^N \mathbf{A}_{1n}(\tilde{\boldsymbol{\alpha}} - \boldsymbol{\eta}^\alpha) \mathbf{t}_n \\
&= \mathbf{t}_1 + \sum_{n=2}^N \mathbf{A}_{1n}(\tilde{\boldsymbol{\alpha}} - \boldsymbol{\eta}^\alpha) \mathbf{t}_n \\
&\stackrel{\text{eq. (13)}}{=} \mathbf{t}_1 + \sum_{n=2}^N \left[ \mathbf{A}_{1n}(\tilde{\boldsymbol{\alpha}}) \left( \prod_{k=1}^{n-1} \text{Exp} \left( -\mathbf{A}_{k+1,n}^\top(\tilde{\boldsymbol{\alpha}}) \boldsymbol{\eta}_k^{\alpha\top} \right) \right) \mathbf{t}_n \right] \\
&= \mathbf{t}_1 + \sum_{n=2}^N [\mathbf{A}_{1n}(\tilde{\boldsymbol{\alpha}}) \text{Exp}(-\delta \mathbf{f}_R^n) \mathbf{t}_n]
\end{aligned} \tag{11}$$

where  $\delta \mathbf{f}_R^n$  represents the cumulative rotational noise of frame  $n$ . This can be compared to  $\delta \mathbf{f}_R$  in (9) which represents the full rotational noise of the contact pose, frame  $N+1$ . Now, using the same first-order approximations used in (9), we can approximate (1.2) as:

$$\begin{aligned}
\mathbf{R}^\top(\mathbf{d} - \mathbf{p}) &\approx \mathbf{t}_1 + \sum_{n=2}^N \left[ \mathbf{A}_{1n}(\tilde{\boldsymbol{\alpha}}) \text{Exp} \left( -\sum_{k=1}^{n-1} \mathbf{A}_{k+1,n}^\top(\tilde{\boldsymbol{\alpha}}) \boldsymbol{\eta}_k^{\alpha\top} \right) \mathbf{t}_n \right] \\
&\approx \mathbf{t}_1 + \sum_{n=2}^N \left[ \mathbf{A}_{1n}(\tilde{\boldsymbol{\alpha}}) \left( \mathbf{I} - \left( \sum_{k=1}^{n-1} \mathbf{A}_{k+1,n}^\top(\tilde{\boldsymbol{\alpha}}) \boldsymbol{\eta}_k^{\alpha\top} \right)^\wedge \right) \mathbf{t}_n \right] \\
&= \mathbf{t}_1 + \sum_{n=2}^N \left[ \mathbf{A}_{1n}(\tilde{\boldsymbol{\alpha}}) \mathbf{t}_n - \mathbf{A}_{1n}(\tilde{\boldsymbol{\alpha}}) \left( \sum_{k=1}^{n-1} \left( \mathbf{A}_{k+1,n}^\top(\tilde{\boldsymbol{\alpha}}) \boldsymbol{\eta}_k^{\alpha\top} \right)^\wedge \right) \mathbf{t}_n \right] \\
&= \mathbf{t}_1 + \sum_{n=2}^N \left[ \mathbf{A}_{1n}(\tilde{\boldsymbol{\alpha}}) \mathbf{t}_n + \mathbf{A}_{1n}(\tilde{\boldsymbol{\alpha}}) \mathbf{t}_n^\wedge \sum_{k=1}^{n-1} \mathbf{A}_{k+1,n}^\top(\tilde{\boldsymbol{\alpha}}) \boldsymbol{\eta}_k^{\alpha\top} \right] \\
&= \sum_{n=1}^N \mathbf{A}_{1n}(\tilde{\boldsymbol{\alpha}}) \mathbf{t}_n + \sum_{n=2}^N \left[ \mathbf{A}_{1n}(\tilde{\boldsymbol{\alpha}}) \mathbf{t}_n^\wedge \sum_{k=1}^{n-1} \mathbf{A}_{k+1,n}^\top(\tilde{\boldsymbol{\alpha}}) \boldsymbol{\eta}_k^{\alpha\top} \right] \\
&= \mathbf{f}_p(\tilde{\boldsymbol{\alpha}}) + \sum_{n=2}^N \left[ \mathbf{A}_{1n}(\tilde{\boldsymbol{\alpha}}) \mathbf{t}_n^\wedge \sum_{k=1}^{n-1} \mathbf{A}_{k+1,n}^\top(\tilde{\boldsymbol{\alpha}}) \boldsymbol{\eta}_k^{\alpha\top} \right]
\end{aligned} \tag{12}$$

By expanding and recollecting terms, the summations can be grouped:

$$\begin{aligned}
\mathbf{R}^\top(\mathbf{d} - \mathbf{p}) &= \mathbf{f}_p(\tilde{\alpha}) + \mathbf{A}_{1,2}(\tilde{\alpha})\mathbf{t}_2^\wedge \left( \mathbf{A}_{2,2}^\top(\tilde{\alpha})\boldsymbol{\eta}_1^{\alpha^\dagger} \right) \\
&\quad + \mathbf{A}_{1,3}(\tilde{\alpha})\mathbf{t}_3^\wedge \left( \mathbf{A}_{2,3}^\top(\tilde{\alpha})\boldsymbol{\eta}_1^{\alpha^\dagger} + \mathbf{A}_{3,3}^\top(\tilde{\alpha})\boldsymbol{\eta}_2^{\alpha^\dagger} \right) \\
&\quad \vdots \\
&\quad + \mathbf{A}_{1,N}(\tilde{\alpha})\mathbf{t}_N^\wedge \left( \mathbf{A}_{2,N}^\top(\tilde{\alpha})\boldsymbol{\eta}_1^{\alpha^\dagger} + \mathbf{A}_{3,N}^\top(\tilde{\alpha})\boldsymbol{\eta}_2^{\alpha^\dagger} + \cdots + \mathbf{A}_{N,N}^\top(\tilde{\alpha})\boldsymbol{\eta}_{N-1}^{\alpha^\dagger} \right) \\
&= \mathbf{f}_p(\tilde{\alpha}) + \left( \mathbf{A}_{1,2}(\tilde{\alpha})\mathbf{t}_2^\wedge \mathbf{A}_{2,2}^\top(\tilde{\alpha}) + \mathbf{A}_{1,3}(\tilde{\alpha})\mathbf{t}_3^\wedge \mathbf{A}_{2,3}^\top(\tilde{\alpha}) + \cdots + \mathbf{A}_{1,N}(\tilde{\alpha})\mathbf{t}_N^\wedge \mathbf{A}_{2,N}^\top(\tilde{\alpha}) \right) \boldsymbol{\eta}_1^{\alpha^\dagger} \\
&\quad + \left( \mathbf{A}_{1,3}(\tilde{\alpha})\mathbf{t}_3^\wedge \mathbf{A}_{3,3}^\top(\tilde{\alpha}) + \cdots + \mathbf{A}_{1,N}(\tilde{\alpha})\mathbf{t}_N^\wedge \mathbf{A}_{3,N}^\top(\tilde{\alpha}) \right) \boldsymbol{\eta}_2^{\alpha^\dagger} \\
&\quad + \left( \mathbf{A}_{1,N}(\tilde{\alpha})\mathbf{t}_N^\wedge \mathbf{A}_{N,N}^\top(\tilde{\alpha}) \right) \boldsymbol{\eta}_{N-1}^{\alpha^\dagger} \\
&= \mathbf{f}_p(\tilde{\alpha}) + \sum_{k=1}^{N-1} \sum_{n=k}^{N-1} \mathbf{A}_{1,n+1}(\tilde{\alpha})\mathbf{t}_{n+1}^\wedge \mathbf{A}_{k+1,n+1}^\top(\tilde{\alpha})\boldsymbol{\eta}_k^{\alpha^\dagger} \\
&\triangleq \mathbf{f}_p(\tilde{\alpha}) - \delta \mathbf{f}_p
\end{aligned} \tag{13}$$

where the noise term,  $\delta \mathbf{f}_p$ , is a sum of zero-mean Gaussians, and is therefore also a zero-mean Gaussian.  $\square$

The forward kinematics measurement model can now be defined as:

$$\begin{aligned}
\mathbf{f}_R(\tilde{\alpha}) &= \mathbf{R}^\top \mathbf{C} \text{Exp}(\delta \mathbf{f}_R) \\
\mathbf{f}_p(\tilde{\alpha}) &= \mathbf{R}^\top(\mathbf{d} - \mathbf{p}) + \delta \mathbf{f}_p
\end{aligned} \tag{14}$$

with the noise characterized by:

$$\begin{bmatrix} \delta \mathbf{f}_R \\ \delta \mathbf{f}_p \end{bmatrix} = \begin{bmatrix} \sum_{k=1}^{N-1} \mathbf{A}_{k+1,N+1}^\top(\tilde{\alpha})\boldsymbol{\eta}_k^{\alpha^\dagger} \\ \sum_{k=1}^{N-1} \sum_{n=k}^{N-1} -\mathbf{A}_{1,n+1}(\tilde{\alpha})\mathbf{t}_{n+1}^\wedge \mathbf{A}_{k+1,n+1}^\top(\tilde{\alpha})\boldsymbol{\eta}_k^{\alpha^\dagger} \end{bmatrix} \sim \mathcal{N}(\mathbf{0}_{6,1}, \boldsymbol{\Sigma}_{\mathcal{F}}) \tag{15}$$

### 1.3 Residuals and Covariance

After the noise is separated out from the measurement equations, the forward kinematic residual errors can be written as:

$$\begin{aligned}
\mathbf{r}_{f_R} &= \text{Log} \left( \mathbf{f}_R(\tilde{\alpha}_i)^\top \mathbf{R}_i^\top \mathbf{C}_i \right) \\
\mathbf{r}_{f_p} &= \mathbf{R}_i^\top(\mathbf{d}_i - \mathbf{p}_i) - \mathbf{f}_p(\tilde{\alpha}_i)
\end{aligned} \tag{16}$$

In addition, the forward kinematics noise can be rewritten as a linear system:

$$\begin{bmatrix} \delta \mathbf{f}_R \\ \delta \mathbf{f}_p \end{bmatrix} = \begin{bmatrix} \mathbf{Q}(\tilde{\alpha}_i) \\ \mathbf{S}(\tilde{\alpha}_i) \end{bmatrix} \begin{bmatrix} \boldsymbol{\eta}_1^{\alpha^\dagger} \\ \boldsymbol{\eta}_2^{\alpha^\dagger} \\ \vdots \\ \boldsymbol{\eta}_{N-1}^{\alpha^\dagger} \end{bmatrix} \tag{17}$$

where columns of the  $3 \times 3(N-1)$  matrices  $\mathbf{Q}$  and  $\mathbf{S}$  are derived from Eq (15):

$$\begin{aligned}
\mathbf{Q}_i(\tilde{\alpha}) &= \mathbf{A}_{i+1,N+1}^\top(\tilde{\alpha}) \\
\mathbf{S}_i(\tilde{\alpha}) &= - \sum_{n=i}^{N-1} \mathbf{A}_{1,n+1}(\tilde{\alpha})\mathbf{t}_{n+1}^\wedge \mathbf{A}_{i+1,n+1}^\top(\tilde{\alpha})
\end{aligned} \tag{18}$$

The covariance can be computed using the linear noise model, Eq (17) , and the sensor covariance matrix,  $\Sigma_{\alpha^\dagger} \in \mathbb{R}^{3(N-1) \times 3(N-1)}$ , that describes the encoder noise  $\eta^{\alpha^\dagger}$ :

$$\Sigma_{\mathcal{F}_i} = \begin{bmatrix} \mathbf{Q}(\tilde{\alpha}_i) \\ \mathbf{S}(\tilde{\alpha}_i) \end{bmatrix} \Sigma_{\alpha^\dagger} [\mathbf{Q}^\top(\tilde{\alpha}_i) \quad \mathbf{S}^\top(\tilde{\alpha}_i)] \quad (19)$$

## 2 Forward Kinematic Factor Jacobians

Given a retraction mapping and the associated manifold, we can optimize over the manifold by iteratively *lifting* the cost function of our optimization problem to the tangent space, solving the reparameterized problem, and then mapping the updated solution back to the manifold using the retraction. For SE(3) we adopt the retraction used in [2],  $\mathcal{R}_T(\delta\phi, \delta\mathbf{p}) = (\mathbf{R}\text{Exp}(\delta\phi), \mathbf{p} + \mathbf{R}\delta\phi)$ ,  $\text{vec}(\delta\phi, \delta\mathbf{p}) \in \mathbb{R}^6$ .

Therefore, lifting involves the following retraction on the base and the contact frame poses:

$$\begin{aligned} \mathbf{R}_i &\leftarrow \mathbf{R}_i \text{Exp}(\delta\phi_i) & \mathbf{C}_i &\leftarrow \mathbf{C}_i \text{Exp}(\delta\theta_i) \\ \mathbf{p}_i &\leftarrow \mathbf{p}_i + \mathbf{R}_i \delta\mathbf{p}_i & \mathbf{d}_i &\leftarrow \mathbf{d}_i + \mathbf{C}_i \delta\mathbf{d}_i \end{aligned} \quad (20)$$

The Jacobians for the forward kinematic factors are derived in the following sections.

### 2.1 Jacobians of $\mathbf{r}_{f_R}$

The Jacobians of the forward kinematic factor residuals can now be computed as:

$$\begin{aligned} \mathbf{r}_{f_R}(\mathbf{R}_i \text{Exp}(\delta\phi_i)) &= \text{Log}(\mathbf{f}_R(\tilde{\alpha}_i)^\top (\mathbf{R}_i \text{Exp}(\delta\phi_i))^\top \mathbf{C}_i) \\ &= \text{Log}(\mathbf{f}_R(\tilde{\alpha}_i)^\top \text{Exp}(-\delta\phi_i) \mathbf{R}_i^\top \mathbf{C}_i) \\ &= \text{Log}(\mathbf{f}_R(\tilde{\alpha}_i)^\top \mathbf{R}_i^\top \mathbf{C}_i \text{Exp}(-\mathbf{C}_i^\top \mathbf{R}_i \delta\phi_i)) \\ &= \text{Log}[\text{Exp}(\text{Log}(\mathbf{f}_R(\tilde{\alpha}_i)^\top \mathbf{R}_i^\top \mathbf{C}_i)) \text{Exp}(-\mathbf{C}_i^\top \mathbf{R}_i \delta\phi_i)] \\ &\approx \text{Log}(\mathbf{f}_R(\tilde{\alpha}_i)^\top \mathbf{R}_i^\top \mathbf{C}_i) + \mathbf{J}_r^{-1}(\text{Log}(\mathbf{f}_R(\tilde{\alpha}_i)^\top \mathbf{R}_i^\top \mathbf{C}_i))(-\mathbf{C}_i^\top \mathbf{R}_i \delta\phi_i) \\ &= \mathbf{r}_{f_R}(\mathbf{R}_i) - \mathbf{J}_r^{-1}(\mathbf{r}_{f_R}(\mathbf{R}_i)) \mathbf{C}_i^\top \mathbf{R}_i \delta\phi_i \end{aligned} \quad (21)$$

$$\begin{aligned} \mathbf{r}_{f_R}(\mathbf{C}_i \text{Exp}(\delta\theta_i)) &= \text{Log}(\mathbf{f}_R(\tilde{\alpha}_i)^\top \mathbf{R}_i^\top (\mathbf{C}_i \text{Exp}(\delta\theta_i))) \\ &= \text{Log}[\text{Exp}(\text{Log}(\mathbf{f}_R(\tilde{\alpha}_i)^\top \mathbf{R}_i^\top \mathbf{C}_i)) \text{Exp}(\delta\theta_i)] \\ &\approx \text{Log}(\mathbf{f}_R(\tilde{\alpha}_i)^\top \mathbf{R}_i^\top \mathbf{C}_i) + \mathbf{J}_r^{-1}(\text{Log}(\mathbf{f}_R(\tilde{\alpha}_i)^\top \mathbf{R}_i^\top \mathbf{C}_i)) \delta\theta_i \\ &= \mathbf{r}_{f_R}(\mathbf{C}_i) + \mathbf{J}_r^{-1}(\mathbf{r}_{f_R}(\mathbf{C}_i)) \delta\theta_i \end{aligned} \quad (22)$$

$$\begin{aligned} \frac{\partial \mathbf{r}_{f_R}}{\partial \delta\phi_i} &= -\mathbf{J}_r^{-1}(\mathbf{r}_{f_R}(\mathbf{R}_i)) \mathbf{C}_i^\top \mathbf{R}_i \\ \frac{\partial \mathbf{r}_{f_R}}{\partial \delta\mathbf{p}_i} &= \mathbf{0}_{3,3} \\ \frac{\partial \mathbf{r}_{f_R}}{\partial \delta\theta_i} &= \mathbf{J}_r^{-1}(\mathbf{r}_{f_R}(\mathbf{C}_i)) \\ \frac{\partial \mathbf{r}_{f_R}}{\partial \delta\mathbf{d}_i} &= \mathbf{0}_{3,3} \end{aligned} \quad (23)$$

## 2.2 Jacobians of $\mathbf{r}_{f_p}$

$$\begin{aligned}
\mathbf{r}_{f_p}(\mathbf{R}_i \text{Exp}(\delta\phi_i)) &= (\mathbf{R}_i \text{Exp}(\delta\phi_i))^\top (\mathbf{d}_i - \mathbf{p}_i) - \mathbf{f}_p(\tilde{\alpha}_i) \\
&= \text{Exp}(-\delta\phi_i) \mathbf{R}_i^\top (\mathbf{d}_i - \mathbf{p}_i) - \mathbf{f}_p(\tilde{\alpha}_i) \\
&\approx (\mathbf{I} - \delta\phi_i^\wedge) \mathbf{R}_i^\top (\mathbf{d}_i - \mathbf{p}_i) - \mathbf{f}_p(\tilde{\alpha}_i) \\
&= \mathbf{R}_i^\top (\mathbf{d}_i - \mathbf{p}_i) - \delta\phi_i^\wedge \mathbf{R}_i^\top (\mathbf{d}_i - \mathbf{p}_i) - \mathbf{f}_p(\tilde{\alpha}_i) \\
&= \mathbf{R}_i^\top (\mathbf{d}_i - \mathbf{p}_i) - \mathbf{f}_p(\tilde{\alpha}_i) + (\mathbf{R}_i^\top (\mathbf{d}_i - \mathbf{p}_i))^\wedge \delta\phi_i \\
&= \mathbf{r}_{f_p}(\mathbf{R}_i) + \left( \mathbf{R}_i^\top (\mathbf{d}_i - \mathbf{p}_i) \right)^\wedge \delta\phi_i
\end{aligned} \tag{24}$$

$$\begin{aligned}
\mathbf{r}_{f_p}(\mathbf{p}_i + \mathbf{R}_i \delta\mathbf{p}_i) &= \mathbf{R}_i^\top (\mathbf{d}_i - (\mathbf{p}_i + \mathbf{R}_i \delta\mathbf{p}_i)) - \mathbf{f}_p(\tilde{\alpha}_i) \\
&= \mathbf{R}_i^\top (\mathbf{d}_i - \mathbf{p}_i - \mathbf{R}_i \delta\mathbf{p}_i) - \mathbf{f}_p(\tilde{\alpha}_i) \\
&= \mathbf{R}_i^\top (\mathbf{d}_i - \mathbf{p}_i) - \delta\mathbf{p}_i - \mathbf{f}_p(\tilde{\alpha}_i) \\
&= \mathbf{R}_i^\top (\mathbf{d}_i - \mathbf{p}_i) - \mathbf{f}_p(\tilde{\alpha}_i) - \delta\mathbf{p}_i \\
&= \mathbf{r}_{f_p}(\mathbf{p}_i) - \delta\mathbf{p}_i
\end{aligned} \tag{25}$$

$$\begin{aligned}
\mathbf{r}_{f_p}(\mathbf{d}_i + \mathbf{C}_i \delta\mathbf{d}_i) &= \mathbf{R}_i^\top ((\mathbf{d}_i + \mathbf{C}_i \delta\mathbf{d}_i) - \mathbf{p}_i) - \mathbf{f}_p(\tilde{\alpha}_i) \\
&= \mathbf{R}_i^\top (\mathbf{d}_i + \mathbf{C}_i \delta\mathbf{d}_i - \mathbf{p}_i) - \mathbf{f}_p(\tilde{\alpha}_i) \\
&= \mathbf{R}_i^\top (\mathbf{d}_i - \mathbf{p}_i) + \mathbf{R}_i^\top \mathbf{C}_i \delta\mathbf{d}_i - \mathbf{f}_p(\tilde{\alpha}_i) \\
&= \mathbf{R}_i^\top (\mathbf{d}_i - \mathbf{p}_i) - \mathbf{f}_p(\tilde{\alpha}_i) + \mathbf{R}_i^\top \mathbf{C}_i \delta\mathbf{d}_i \\
&= \mathbf{r}_{f_p}(\mathbf{d}_i) + \mathbf{R}_i^\top \mathbf{C}_i \delta\mathbf{d}_i
\end{aligned} \tag{26}$$

$$\begin{aligned}
\frac{\partial \mathbf{r}_{f_p}}{\partial \delta\phi_i} &= \left( \mathbf{R}_i^\top (\mathbf{d}_i - \mathbf{p}_i) \right)^\wedge \\
\frac{\partial \mathbf{r}_{f_p}}{\partial \delta\mathbf{p}_i} &= -\mathbf{I}_3 \\
\frac{\partial \mathbf{r}_{f_p}}{\partial \delta\boldsymbol{\theta}_i} &= \mathbf{0}_{3,3} \\
\frac{\partial \mathbf{r}_{f_p}}{\partial \delta\mathbf{d}_i} &= \mathbf{R}_i^\top \mathbf{C}_i
\end{aligned} \tag{27}$$

## 3 Rigid Contact Factor Derivations

### 3.1 Measurement Model

Starting with (29), the relative motion increments for the contact frame are given by:

$$\begin{aligned}
\Delta \mathbf{C}_{ij} &= \mathbf{C}_i^\top \mathbf{C}_j = \prod_{k=i}^{j-1} \text{Exp}(\boldsymbol{\eta}_k^{\omega_d} \Delta t) \\
\Delta \mathbf{d}_{ij} &= \mathbf{C}_i^\top (\mathbf{d}_j - \mathbf{d}_i) = \sum_{k=i}^{j-1} \Delta \mathbf{C}_{ik} \boldsymbol{\eta}_k^{v_d} \Delta t
\end{aligned} \tag{28}$$

Next, we wish to isolate the noise terms. First, we will deal with the rotation of the contact frame. The product of multiple incremental rotations can be expressed as one larger rotation. Therefore,

$$\Delta \mathbf{C}_{ij} \triangleq \tilde{\Delta \mathbf{C}}_{ij} \text{Exp}(-\delta\boldsymbol{\theta}_{ij}) \tag{29}$$

where  $\Delta\tilde{\mathbf{C}}_{ij}$  denotes the measured relative rotation of the contact frame between times  $t_i$  and  $t_j$ . Due to the rigid contact frame assumption,  $\Delta\tilde{\mathbf{C}}_{ij} = \mathbf{I}$ . The noise term  $\delta\boldsymbol{\theta}_{ij} = -\prod_{k=i}^{j-1} \text{Exp}(\boldsymbol{\eta}_k^{\omega d} \Delta t)$  accounts for the accumulated angular contact slip. Though repeated first order approximation,  $\delta\boldsymbol{\theta}_{ij}$  is shown to be approximately zero mean and Gaussian:

$$\begin{aligned}
\delta\boldsymbol{\theta}_{ij} &= -\text{Log} \left( \prod_{k=i}^{j-1} -\text{Exp}(\boldsymbol{\eta}_k^{\omega d} \Delta t) \right) \\
&= -\text{Log} \left( \text{Exp} \left( \text{Log} \left( \prod_{k=i}^{j-2} -\text{Exp}(\boldsymbol{\eta}_k^{\omega d} \Delta t) \right) \right) \text{Exp}(-\boldsymbol{\eta}_{j-1}^{\omega d} \Delta t) \right) \\
&\stackrel{\text{eq. (2)}}{\approx} -\text{Log} \left( \prod_{k=i}^{j-2} -\text{Exp}(\boldsymbol{\eta}_k^{\omega d} \Delta t) \right) + \mathbf{J}_r^{-1} \left( \text{Log} \left( \prod_{k=i}^{j-2} -\text{Exp}(\boldsymbol{\eta}_k^{\omega d} \Delta t) \right) \right) \boldsymbol{\eta}_{j-1}^{\omega d} \Delta t \\
&\approx -\text{Log} \left( \prod_{k=i}^{j-2} \text{Exp}(\boldsymbol{\eta}_k^{\omega d} \Delta t) \right) + \boldsymbol{\eta}_{j-1}^{\omega d} \Delta t \\
&\vdots \\
&\approx \sum_{k=i}^{j-1} \boldsymbol{\eta}_k^{\omega d} \Delta t
\end{aligned} \tag{30}$$

where we make use of the fact that for small noise quantities, the right Jacobian and its inverse are close to the identity.

Now, we can isolate the noise in the position of the contact frame by substituting (29) into  $\Delta\mathbf{d}_{ij}$ , using the first-order exponential map approximation, and dropping the higher order noise terms.

$$\begin{aligned}
\Delta\mathbf{d}_{ij} &\approx \sum_{k=i}^{j-1} \Delta\tilde{\mathbf{C}}_{ik} (\mathbf{I} - \delta\boldsymbol{\theta}_{ik}^\wedge) \boldsymbol{\eta}_k^{vd} \Delta t \\
&= \sum_{k=i}^{j-1} (\mathbf{I} - \delta\boldsymbol{\theta}_{ik}^\wedge) \boldsymbol{\eta}_k^{vd} \Delta t \\
&\approx -\sum_{k=i}^{j-1} \boldsymbol{\eta}_k^{vd} \Delta t \\
&\triangleq \Delta\tilde{\mathbf{d}}_{ij} - \delta\mathbf{d}_{ij}
\end{aligned} \tag{31}$$

where  $\Delta\tilde{\mathbf{d}}_{ij}$  denotes the measured incremental translation of the contact frame between times  $t_i$  and  $t_j$ . Again, due to the rigid contact frame assumption,  $\Delta\tilde{\mathbf{d}}_{ij} = \mathbf{0}$ . The noise term  $\delta\mathbf{d}_{ij} = \sum_{k=i}^{j-1} \boldsymbol{\eta}_k^{vd} \Delta t$  is a linear combination of Gaussians, and is therefore also zero mean and Gaussian.

Finally, we arrive at the *preintegrated contact measurement model*:

$$\begin{aligned}
\Delta\tilde{\mathbf{C}}_{ij} &= \mathbf{C}_i^\top \mathbf{C}_j \text{Exp}(\delta\boldsymbol{\theta}_{ij}) = \mathbf{I}_3 \\
\Delta\tilde{\mathbf{d}}_{ij} &= \mathbf{C}_i^\top (\mathbf{d}_j - \mathbf{d}_i) + \delta\mathbf{d}_{ij} = \mathbf{0}_{3,1}
\end{aligned} \tag{32}$$

with the noise characterized by:

$$\begin{bmatrix} \delta\boldsymbol{\theta}_{ij} \\ \delta\mathbf{d}_{ij} \end{bmatrix} = \begin{bmatrix} \sum_{k=i}^{j-1} \boldsymbol{\eta}_k^{\omega d} \Delta t \\ \sum_{k=i}^{j-1} \boldsymbol{\eta}_k^{vd} \Delta t \end{bmatrix} \sim \mathcal{N}(\mathbf{0}_{6,1}, \boldsymbol{\Sigma}_{\mathcal{C}_{ij}}) \tag{33}$$

### 3.2 Residuals and Covariance

Once the noise terms are separated out, we can write down the residual errors:

$$\begin{aligned}\mathbf{r}_{\Delta\mathbf{C}_{ij}} &= \text{Log}(\mathbf{C}_i^\top \mathbf{C}_j) \\ \mathbf{r}_{\Delta\mathbf{d}_{ij}} &= \mathbf{C}_i^\top (\mathbf{d}_j - \mathbf{d}_i)\end{aligned}\tag{34}$$

Furthermore, since both noise terms are simply additive Gaussians, the covariance can easily be computed. Written as a linear system, the measurement noise model becomes:

$$\begin{bmatrix} \delta\boldsymbol{\theta}_{ik+1} \\ \delta\mathbf{d}_{ik+1} \end{bmatrix} = \begin{bmatrix} \delta\boldsymbol{\theta}_{ik} \\ \delta\mathbf{d}_{ik} \end{bmatrix} + \Delta t \begin{bmatrix} \boldsymbol{\eta}_k^{\omega d} \\ \boldsymbol{\eta}_k^{vd} \end{bmatrix}\tag{35}$$

This allows us to compute the covariance as iteratively starting at  $\boldsymbol{\Sigma}_{\mathcal{C}_{ii}} = 0$ :

$$\boldsymbol{\Sigma}_{\mathcal{C}_{ik+1}} = \boldsymbol{\Sigma}_{\mathcal{C}_{ik}} + \begin{bmatrix} \boldsymbol{\Sigma}_{\omega d} & \mathbf{0}_{3,3} \\ \mathbf{0}_{3,3} & \boldsymbol{\Sigma}_{vd} \end{bmatrix} \Delta t^2\tag{36}$$

where  $\boldsymbol{\Sigma}_{\boldsymbol{\eta}^{\omega d}}$  and  $\boldsymbol{\Sigma}_{\boldsymbol{\eta}^{vd}}$  are the discrete covariance matrices of the contact frame's angular and linear velocity noises,  $\boldsymbol{\eta}^{\omega d}$  and  $\boldsymbol{\eta}^{vd}$ . This iterative update equation allows for time-varying contact noise. This would be particularly useful if the noise was modeled to depend on contact pressure.

If the contact noise kept constant, (36) simply becomes:

$$\boldsymbol{\Sigma}_{\mathcal{C}_{ij}} = \begin{bmatrix} \boldsymbol{\Sigma}_{\omega} & \mathbf{0}_{3,3} \\ \mathbf{0}_{3,3} & \boldsymbol{\Sigma}_v \end{bmatrix} \Delta t_{ij}\tag{37}$$

where  $\boldsymbol{\Sigma}_{\boldsymbol{\eta}^{\omega}}$  and  $\boldsymbol{\Sigma}_{\boldsymbol{\eta}^v}$  are the continuous covariance matrices of the contact frame's angular and linear velocity noises,  $\boldsymbol{\eta}^{\omega}$  and  $\boldsymbol{\eta}^v$ , and  $\Delta t_{ij} = \sum_{k=i}^j \Delta t$ .

## 4 Rigid Contact Factor Jacobians

### 4.1 Jacobians of $\mathbf{r}_{\Delta\mathbf{C}_{ij}}$

Using the retraction defined in 20, the Jacobians of the rigid contact factor residuals can now be computed as:

$$\begin{aligned}\mathbf{r}_{\Delta\mathbf{C}_{ij}}(\mathbf{C}_i \text{Exp}(\delta\boldsymbol{\theta}_i)) &= \text{Log}((\mathbf{C}_i \text{Exp}(\delta\boldsymbol{\theta}_i))^\top \mathbf{C}_j) \\ &= \text{Log}(\text{Exp}(-\delta\boldsymbol{\theta}_i) \mathbf{C}_i^\top \mathbf{C}_j) \\ &= \text{Log}(\mathbf{C}_i^\top \mathbf{C}_j \text{Exp}(-\mathbf{C}_j^\top \mathbf{C}_i \delta\boldsymbol{\theta}_i)) \\ &= \text{Log}(\text{Exp}(\text{Log}(\mathbf{C}_i^\top \mathbf{C}_j)) \text{Exp}(-\mathbf{C}_j^\top \mathbf{C}_i \delta\boldsymbol{\theta}_i)) \\ &= \text{Log}(\mathbf{C}_i^\top \mathbf{C}_j) + \mathbf{J}_r^{-1}(\text{Log}(\mathbf{C}_i^\top \mathbf{C}_j))(-\mathbf{C}_j^\top \mathbf{C}_i \delta\boldsymbol{\theta}_i) \\ &= \mathbf{r}_{\Delta\mathbf{C}_{ij}}(\mathbf{C}_i) - \mathbf{J}_r^{-1}(\mathbf{r}_{\Delta\mathbf{C}_{ij}}(\mathbf{C}_i)) \mathbf{C}_j^\top \mathbf{C}_i \delta\boldsymbol{\theta}_i\end{aligned}\tag{38}$$

$$\begin{aligned}\mathbf{r}_{\Delta\mathbf{C}_{ij}}(\mathbf{C}_j \text{Exp}(\delta\boldsymbol{\theta}_j)) &= \text{Log}(\mathbf{C}_i^\top (\mathbf{C}_j \text{Exp}(\delta\boldsymbol{\theta}_j))) \\ &= \text{Log}(\mathbf{C}_i^\top \mathbf{C}_j \text{Exp}(\delta\boldsymbol{\theta}_j)) \\ &= \text{Log}(\text{Exp}(\text{Log}(\mathbf{C}_i^\top \mathbf{C}_j)) \text{Exp}(\delta\boldsymbol{\theta}_j)) \\ &= \text{Log}(\mathbf{C}_i^\top \mathbf{C}_j) + \mathbf{J}_r^{-1}(\text{Log}(\mathbf{C}_i^\top \mathbf{C}_j)) \delta\boldsymbol{\theta}_j \\ &= \mathbf{r}_{\Delta\mathbf{C}_{ij}}(\mathbf{C}_j) + \mathbf{J}_r^{-1}(\mathbf{r}_{\Delta\mathbf{C}_{ij}}(\mathbf{C}_j)) \delta\boldsymbol{\theta}_j\end{aligned}\tag{39}$$

Written concisely, the Jacobians of  $\mathbf{r}_{\Delta \mathbf{C}_{ij}}$  are,

$$\begin{aligned}
\frac{\partial \mathbf{r}_{\Delta \mathbf{C}_{ij}}}{\partial \delta \boldsymbol{\theta}_i} &= -\mathbf{J}_r^{-1}(\mathbf{r}_{\Delta \mathbf{C}_{ij}}(\mathbf{C}_i)) \mathbf{C}_j^\top \mathbf{C}_i \\
\frac{\partial \mathbf{r}_{\Delta \mathbf{C}_{ij}}}{\partial \delta \mathbf{d}_i} &= \mathbf{0}_{3,3} \\
\frac{\partial \mathbf{r}_{\Delta \mathbf{C}_{ij}}}{\partial \delta \boldsymbol{\theta}_j} &= \mathbf{J}_r^{-1}(\mathbf{r}_{\Delta \mathbf{C}_{ij}}(\mathbf{C}_j)) \\
\frac{\partial \mathbf{r}_{\Delta \mathbf{C}_{ij}}}{\partial \delta \mathbf{d}_j} &= \mathbf{0}_{3,3}
\end{aligned} \tag{40}$$

## 4.2 Jacobians of $\mathbf{r}_{\Delta \mathbf{d}_{ij}}$

$$\begin{aligned}
\mathbf{r}_{\Delta \mathbf{d}_{ij}}(\mathbf{C}_i \text{Exp}(\delta \boldsymbol{\theta}_i)) &= (\mathbf{C}_i \text{Exp}(\delta \boldsymbol{\theta}_i))^\top (\mathbf{d}_j - \mathbf{d}_i) \\
&= \text{Exp}(-\delta \boldsymbol{\theta}_i) \mathbf{C}_i^\top (\mathbf{d}_j - \mathbf{d}_i) \\
&\approx (\mathbf{I} - \delta \boldsymbol{\theta}_i^\wedge) \mathbf{C}_i^\top (\mathbf{d}_j - \mathbf{d}_i) \\
&\approx \mathbf{C}_i^\top (\mathbf{d}_j - \mathbf{d}_i) - \delta \boldsymbol{\theta}_i^\wedge \mathbf{C}_i^\top (\mathbf{d}_j - \mathbf{d}_i) \\
&\approx \mathbf{C}_i^\top (\mathbf{d}_j - \mathbf{d}_i) + (\mathbf{C}_i^\top (\mathbf{d}_j - \mathbf{d}_i))^\wedge \delta \boldsymbol{\theta}_i \\
&= \mathbf{r}_{\Delta \mathbf{d}_{ij}}(\mathbf{C}_i) + (\mathbf{C}_i^\top (\mathbf{d}_j - \mathbf{d}_i))^\wedge \delta \boldsymbol{\theta}_i
\end{aligned} \tag{41}$$

$$\begin{aligned}
\mathbf{r}_{\Delta \mathbf{d}_{ij}}(\mathbf{d}_i + \mathbf{C}_i \delta \mathbf{d}_i) &= \mathbf{C}_i^\top (\mathbf{d}_j - (\mathbf{d}_i + \mathbf{C}_i \delta \mathbf{d}_i)) \\
&= \mathbf{C}_i^\top (\mathbf{d}_j - \mathbf{d}_i - \mathbf{C}_i \delta \mathbf{d}_i) \\
&= \mathbf{C}_i^\top (\mathbf{d}_j - \mathbf{d}_i) - \delta \mathbf{d}_i \\
&= \mathbf{r}_{\Delta \mathbf{d}_{ij}}(\mathbf{d}_i) - \delta \mathbf{d}_i
\end{aligned} \tag{42}$$

$$\begin{aligned}
\mathbf{r}_{\Delta \mathbf{d}_{ij}}(\mathbf{d}_j + \mathbf{C}_j \delta \mathbf{d}_j) &= \mathbf{C}_i^\top ((\mathbf{d}_j + \mathbf{C}_j \delta \mathbf{d}_j) - \mathbf{d}_i) \\
&= \mathbf{C}_i^\top (\mathbf{d}_j + \mathbf{C}_j \delta \mathbf{d}_j - \mathbf{d}_i) \\
&= \mathbf{C}_i^\top (\mathbf{d}_j - \mathbf{d}_i) + \mathbf{C}_i^\top \mathbf{C}_j \delta \mathbf{d}_j \\
&= \mathbf{r}_{\Delta \mathbf{d}_{ij}}(\mathbf{d}_j) + \mathbf{C}_i^\top \mathbf{C}_j \delta \mathbf{d}_j
\end{aligned} \tag{43}$$

Written concisely, the Jacobians of  $\mathbf{r}_{\Delta \mathbf{d}_{ij}}$  are,

$$\begin{aligned}
\frac{\partial \mathbf{r}_{\Delta \mathbf{d}_{ij}}}{\partial \delta \boldsymbol{\theta}_i} &= \left( \mathbf{C}_i^\top (\mathbf{d}_j - \mathbf{d}_i) \right)^\wedge \\
\frac{\partial \mathbf{r}_{\Delta \mathbf{d}_{ij}}}{\partial \delta \mathbf{d}_i} &= -\mathbf{I}_3 \\
\frac{\partial \mathbf{r}_{\Delta \mathbf{d}_{ij}}}{\partial \delta \boldsymbol{\theta}_j} &= \mathbf{0}_{3,3} \\
\frac{\partial \mathbf{r}_{\Delta \mathbf{d}_{ij}}}{\partial \delta \mathbf{d}_j} &= \mathbf{C}_i^\top \mathbf{C}_j
\end{aligned} \tag{44}$$

## 5 Point Contact Factor Derivations

### 5.1 Measurement Model

In this section, we derive the *preintegrated point contact measurement model* beginning with (38).

$$\mathbf{R}_i^\top (\mathbf{d}_j - \mathbf{d}_i) = \mathbf{R}_i^\top \mathbf{C}_i \boldsymbol{\eta}_i^{vd} \Delta t + \sum_{k=i+1}^{j-1} \Delta \mathbf{R}_{ik} \mathbf{f}_R(\tilde{\boldsymbol{\alpha}}_k - \boldsymbol{\eta}_k^\alpha) \boldsymbol{\eta}_k^{vd} \Delta t \quad (45)$$

The rotation increment  $\Delta \mathbf{R}_{ij}$  is defined and explained fully in [2]. In order for this report to be self contained, we include the definitions below.

$$\Delta \mathbf{R}_{ij} \triangleq \mathbf{R}_i^\top \mathbf{R}_j = \prod_{i=1}^{j-1} \text{Exp} \left( (\tilde{\boldsymbol{\omega}}_k - \mathbf{b}_k^g - \boldsymbol{\eta}_k^{gd}) \Delta t \right) = \tilde{\mathbf{R}}_{ij} \text{Exp}(-\delta \phi_{ij}) \quad (46)$$

where up to a first-order approximation,

$$\begin{aligned} \Delta \tilde{\mathbf{R}}_{ij} &= \prod_{i=1}^{j-1} \text{Exp} \left( (\tilde{\boldsymbol{\omega}}_k - \mathbf{b}_k^g) \Delta t \right) \\ \delta \phi_{ij} &\approx \sum_{k=i}^{j-1} \Delta \tilde{\mathbf{R}}_{k+1j}^\top \mathbf{J}_r(\tilde{\boldsymbol{\omega}}_k - \mathbf{b}_k^g) \boldsymbol{\eta}_k^{gd} \Delta T \end{aligned} \quad (47)$$

Substituting (46) into (45) yields,

$$\begin{aligned} \mathbf{R}_i^\top (\mathbf{d}_j - \mathbf{d}_i) &= \mathbf{R}_i^\top \mathbf{C}_i \boldsymbol{\eta}_i^{vd} \Delta t + \sum_{k=i+1}^{j-1} \Delta \tilde{\mathbf{R}}_{ik} \text{Exp}(-\delta \phi_{ik}) \mathbf{f}_R(\tilde{\boldsymbol{\alpha}}_k - \boldsymbol{\eta}_k^\alpha) \boldsymbol{\eta}_k^{vd} \Delta t \\ &\approx \mathbf{R}_i^\top \mathbf{C}_i \boldsymbol{\eta}_i^{vd} \Delta t + \sum_{k=i+1}^{j-1} \Delta \tilde{\mathbf{R}}_{ik} (\mathbf{I} - \phi_{ik}^\wedge) \mathbf{f}_R(\tilde{\boldsymbol{\alpha}}_k - \boldsymbol{\eta}_k^\alpha) \boldsymbol{\eta}_k^{vd} \Delta t \\ &\approx \mathbf{R}_i^\top \mathbf{C}_i \boldsymbol{\eta}_i^{vd} \Delta t + \sum_{k=i+1}^{j-1} \Delta \tilde{\mathbf{R}}_{ik} \mathbf{f}_R(\tilde{\boldsymbol{\alpha}}_k - \boldsymbol{\eta}_k^\alpha) \boldsymbol{\eta}_k^{vd} \Delta t \end{aligned} \quad (48)$$

where all higher order noise terms have been dropped. Substituting in (13) and again dropping higher order noise terms gives:

$$\begin{aligned} \mathbf{R}_i^\top (\mathbf{d}_j - \mathbf{d}_i) &\approx \mathbf{R}_i^\top \mathbf{C}_i \boldsymbol{\eta}_i^{vd} \Delta t + \sum_{k=i+1}^{j-1} \Delta \tilde{\mathbf{R}}_{ik} \left( \mathbf{f}_R(\tilde{\boldsymbol{\alpha}}_k) \prod_{n=1}^{N-1} \text{Exp} \left( -\mathbf{A}_{n+1, N+1}^\top (\tilde{\boldsymbol{\alpha}}) \boldsymbol{\eta}_n^{\alpha^\dagger} \right) \right) \boldsymbol{\eta}_k^{vd} \Delta t \\ &\approx \mathbf{R}_i^\top \mathbf{C}_i \boldsymbol{\eta}_i^{vd} \Delta t + \sum_{k=i+1}^{j-1} \Delta \tilde{\mathbf{R}}_{ik} \left( \mathbf{f}_R(\tilde{\boldsymbol{\alpha}}_k) \prod_{n=1}^{N-1} \left( \mathbf{I} - \left( \mathbf{A}_{n+1, N+1}^\top (\tilde{\boldsymbol{\alpha}}) \boldsymbol{\eta}_n^{\alpha^\dagger} \right)^\wedge \right) \right) \boldsymbol{\eta}_k^{vd} \Delta t \\ &\approx \mathbf{R}_i^\top \mathbf{C}_i \boldsymbol{\eta}_i^{vd} \Delta t + \sum_{k=i+1}^{j-1} \Delta \tilde{\mathbf{R}}_{ik} \left( \mathbf{f}_R(\tilde{\boldsymbol{\alpha}}_k) \left( \mathbf{I} - \sum_{n=1}^{N-1} \left( \mathbf{A}_{n+1, N+1}^\top (\tilde{\boldsymbol{\alpha}}) \boldsymbol{\eta}_n^{\alpha^\dagger} \right)^\wedge \right) \right) \boldsymbol{\eta}_k^{vd} \Delta t \\ &= \mathbf{R}_i^\top \mathbf{C}_i \boldsymbol{\eta}_i^{vd} \Delta t + \sum_{k=i+1}^{j-1} \left[ \Delta \tilde{\mathbf{R}}_{ik} \mathbf{f}_R(\tilde{\boldsymbol{\alpha}}_k) \boldsymbol{\eta}_k^{vd} \Delta t - \Delta \tilde{\mathbf{R}}_{ik} \mathbf{f}_R(\tilde{\boldsymbol{\alpha}}_k) \sum_{n=1}^{N-1} \left( \mathbf{A}_{n+1, N+1}^\top (\tilde{\boldsymbol{\alpha}}) \boldsymbol{\eta}_n^{\alpha^\dagger} \right)^\wedge \boldsymbol{\eta}_k^{vd} \Delta t \right] \\ &\approx \mathbf{R}_i^\top \mathbf{C}_i \boldsymbol{\eta}_i^{vd} \Delta t + \sum_{k=i+1}^{j-1} \Delta \tilde{\mathbf{R}}_{ik} \mathbf{f}_R(\tilde{\boldsymbol{\alpha}}_k) \boldsymbol{\eta}_k^{vd} \Delta t \\ &\triangleq \Delta \tilde{\mathbf{d}}_{ij} - \delta \mathbf{d}_{ij} \end{aligned} \quad (49)$$

where the *preintegrated contact position measurement* is zero, i.e.  $\Delta \tilde{\mathbf{d}}_{ij} = 0$ .

Therefore, up to a first-order approximation, the *preintegrated contact position noise*,  $\delta \mathbf{d}_{ij}$ , does not depend on either the rotational noise,  $\delta \phi_{ij}$ , or the encoder noise,  $\boldsymbol{\eta}^{\alpha \dagger}$ . The *preintegrated point contact measurement model* can now be written as:

$$\Delta \tilde{\mathbf{d}}_{ij} = \mathbf{R}_i^\top (\mathbf{d}_j - \mathbf{d}_i) + \delta \mathbf{d}_{ij} \quad (50)$$

## 5.2 Iterative Noise Propagation

In this section we derive the covariance of the point contact residual function as an iterative update equation. Since the gyroscope measurements are needed to compute  $\delta \mathbf{d}_{ij}$ , the preintegrated point contact factor is formulated as an extension to preintegrated IMU factor described in [2].

The combined IMU / Point Contact preintegration residual includes the three IMU residuals defined in [2] and the new point contact residual, (39). Written explicitly, the full residual becomes:

$$\mathbf{r} = \begin{bmatrix} \mathbf{r}_{\Delta \mathbf{R}_{ij}} \\ \mathbf{r}_{\Delta \mathbf{v}_{ij}} \\ \mathbf{r}_{\Delta \mathbf{p}_{ij}} \\ \mathbf{r}_{\Delta \mathbf{d}_{ij}} \end{bmatrix} = \begin{bmatrix} \text{Log} \left( \left( \Delta \tilde{\mathbf{R}}_{ij}(\bar{\mathbf{b}}_i^g) \text{Exp} \left( \frac{\partial \tilde{\mathbf{R}}_{ij}}{\partial \mathbf{b}^g} \delta \mathbf{b}^g \right) \right)^\top \mathbf{R}_i^\top \mathbf{R}_j \right) \\ \mathbf{R}_i^\top (\mathbf{v}_j - \mathbf{v}_i - \mathbf{g} \Delta t_{ij}) - \left[ \Delta \tilde{\mathbf{v}}_{ij}(\bar{\mathbf{b}}_i^g, \bar{\mathbf{b}}_i^a) + \frac{\partial \tilde{\mathbf{v}}_{ij}}{\partial \mathbf{b}^g} \delta \mathbf{b}^g + \frac{\partial \tilde{\mathbf{v}}_{ij}}{\partial \mathbf{b}^a} \delta \mathbf{b}^a \right] \\ \mathbf{R}_i^\top (\mathbf{p}_j - \mathbf{p}_i - \mathbf{v}_i \Delta t_{ij} - \frac{1}{2} \mathbf{g} \Delta t_{ij}^2) - \left[ \Delta \tilde{\mathbf{p}}_{ij}(\bar{\mathbf{b}}_i^g, \bar{\mathbf{b}}_i^a) + \frac{\partial \tilde{\mathbf{p}}_{ij}}{\partial \mathbf{b}^g} \delta \mathbf{b}^g + \frac{\partial \tilde{\mathbf{p}}_{ij}}{\partial \mathbf{b}^a} \delta \mathbf{b}^a \right] \\ \mathbf{R}_i^\top (\mathbf{d}_j - \mathbf{d}_i) \end{bmatrix} \quad (51)$$

Likewise, the *preintegrated noise vector*, first defined in [2], is appended to include the contact noise yielding:

$$\boldsymbol{\eta}_{ij}^\Delta \triangleq \left[ \delta \phi_{ij}^\top, \delta \mathbf{v}_{ij}^\top, \delta \mathbf{p}_{ij}^\top, \delta \mathbf{d}_{ij}^\top \right]^\top \sim \mathcal{N}(\mathbf{0}_{12,1}, \boldsymbol{\Sigma}_{ij}) \quad (52)$$

The *preintegrated contact position noise*, defined in (49), can be written in an iterative update form by removing a term from the summation and reordering:

$$\begin{aligned} \delta \mathbf{d}_{ij} &= -\mathbf{R}_i^\top \mathbf{C}_i \boldsymbol{\eta}_i^{vd} \Delta t - \sum_{k=i+1}^{j-1} \Delta \tilde{\mathbf{R}}_{ik} \mathbf{f}_R(\tilde{\boldsymbol{\alpha}}_k) \boldsymbol{\eta}_k^{vd} \Delta t \\ &= -\mathbf{R}_i^\top \mathbf{C}_i \boldsymbol{\eta}_i^{vd} \Delta t - \sum_{k=i+1}^{j-2} \Delta \tilde{\mathbf{R}}_{ik} \mathbf{f}_R(\tilde{\boldsymbol{\alpha}}_k) \boldsymbol{\eta}_k^{vd} \Delta t - \Delta \tilde{\mathbf{R}}_{i,j-1} \mathbf{f}_R(\tilde{\boldsymbol{\alpha}}_{j-1}) \boldsymbol{\eta}_{j-1}^{vd} \Delta t \\ &= \delta \mathbf{d}_{ij-1} - \Delta \tilde{\mathbf{R}}_{i,j-1} \mathbf{f}_R(\tilde{\boldsymbol{\alpha}}_{j-1}) \boldsymbol{\eta}_{j-1}^{vd} \Delta t \end{aligned} \quad (53)$$

The iterative update equation can now be written as:

$$\delta \mathbf{d}_{ik+1} = \begin{cases} \delta \mathbf{d}_{ik} - \mathbf{R}_k^\top \mathbf{C}_k \boldsymbol{\eta}_k^{vd} \Delta t & \text{for } k = i \\ \delta \mathbf{d}_{ik} - \Delta \tilde{\mathbf{R}}_{ik} \mathbf{f}_R(\tilde{\boldsymbol{\alpha}}_k) \boldsymbol{\eta}_k^{vd} \Delta t & \text{for } k > i \end{cases} \quad (54)$$

initialized with  $\delta \mathbf{d}_{ii} = \mathbf{0}_{3,1}$ .

Using (54) and the iterative update equations for the rest of  $\boldsymbol{\eta}_{ij}^\Delta$  defined in [2], we can write the linear noise model as:

$$\begin{aligned} \begin{bmatrix} \delta \phi_{ik+1} \\ \delta \mathbf{v}_{ik+1} \\ \delta \mathbf{p}_{ik+1} \\ \delta \mathbf{d}_{ik+1} \end{bmatrix} &= \begin{bmatrix} \Delta \tilde{\mathbf{R}}_{kk+1}^\top & \mathbf{0}_3 & \mathbf{0}_3 & \mathbf{0}_3 \\ -\Delta \tilde{\mathbf{R}}_{ik}(\tilde{\mathbf{a}}_k - \mathbf{b}_i^a)^\wedge \Delta t & \mathbf{I}_3 & \mathbf{0}_3 & \mathbf{0}_3 \\ -\frac{1}{2} \Delta \tilde{\mathbf{R}}_{ik}(\tilde{\mathbf{a}}_k - \mathbf{b}_i^a)^\wedge \Delta t^2 & \mathbf{I}_3 \Delta t & \mathbf{I}_3 & \mathbf{0}_3 \\ \mathbf{0}_3 & \mathbf{0}_3 & \mathbf{0}_3 & \mathbf{I}_3 \end{bmatrix} \begin{bmatrix} \delta \phi_{ik} \\ \delta \mathbf{v}_{ik} \\ \delta \mathbf{p}_{ik} \\ \delta \mathbf{d}_{ik} \end{bmatrix} \\ &+ \begin{bmatrix} \mathbf{J}_r(\tilde{\boldsymbol{\omega}}_k - \mathbf{b}_k^g) \Delta t & \mathbf{0}_3 & \mathbf{0}_3 \\ \mathbf{0}_3 & \Delta \tilde{\mathbf{R}}_{ik} \Delta t & \mathbf{0}_3 \\ \mathbf{0}_3 & \frac{1}{2} \Delta \tilde{\mathbf{R}}_{ik} \Delta t^2 & \mathbf{0}_3 \\ \mathbf{0}_3 & \mathbf{0}_3 & \Delta \tilde{\mathbf{R}}_{ik} \mathbf{f}_R(\tilde{\boldsymbol{\alpha}}_k) \Delta t \end{bmatrix} \begin{bmatrix} \boldsymbol{\eta}_k^{gd} \\ \boldsymbol{\eta}_k^{ad} \\ \boldsymbol{\eta}_k^{vd} \end{bmatrix} \quad \text{for } k > i \end{aligned} \quad (55)$$

This linear system can be simply written as:

$$\boldsymbol{\eta}_{ik+1}^{\Delta} = \mathbf{A}\boldsymbol{\eta}_{ik}^{\Delta} + \mathbf{B}\boldsymbol{\eta}_k^d \quad \text{for } k > i \quad (56)$$

(Note that the update equation for  $k = i$  will be slightly different due to the cases in (54)).

The covariance can now be computed iteratively:

$$\boldsymbol{\Sigma}_{ik+1} = \mathbf{A}\boldsymbol{\Sigma}_{ik}\mathbf{A}^{\top} + \mathbf{B}\boldsymbol{\Sigma}_{\boldsymbol{\eta}}\mathbf{B}^{\top} \quad \text{for } k > i \quad (57)$$

where  $\boldsymbol{\Sigma}_{\boldsymbol{\eta}}$  is the covariance of the raw IMU and contact noise terms  $\boldsymbol{\eta}_k^d$ , initialized with  $\boldsymbol{\Sigma}_{ii} = \mathbf{0}_{12,1}$ .

### 5.3 Separation of IMU and Contact Factors

Upon closer inspection of (55), it can be seen that both  $\mathbf{A}$  and  $\mathbf{B}$  are block diagonal matrices. Therefore, it can also be shown that the final covariance  $\boldsymbol{\Sigma}_{ij}$  will also be block diagonal. This means that the preintegrated point contact measurement is uncorrelated with the preintegrated IMU measurements. In addition, because they are jointly Gaussian, the measurements are independent. This independence is obtained because of the first-order approximation of the noise models.

Since the preintegrated IMU and contact measurements are independent, the combined factor given by (51) can be split into preintegrated IMU factor and a preintegrated contact factor. This separation is important, because existing code implementations of IMU preintegration can be used without modifications.

The separated preintegrated point contact factor residual is simply:

$$\mathbf{r}_{\Delta\mathbf{d}_{ij}} = \mathbf{R}_i^{\top}(\mathbf{d}_j - \mathbf{d}_i) \quad (58)$$

The iterative update equation for the new covariance  $\boldsymbol{\Sigma}_{\mathcal{C}_{ij}} \in \mathbb{R}^{3 \times 3}$  is given by:

$$\boldsymbol{\Sigma}_{\mathcal{C}_{ik+1}} = \begin{cases} \boldsymbol{\Sigma}_{\mathcal{C}_{ik}} + \left(\mathbf{R}_k^{\top}\mathbf{C}_k\Delta t\right)\boldsymbol{\Sigma}_{vd}\left(\mathbf{R}_k^{\top}\mathbf{C}_k\Delta t\right)^{\top} & \text{for } k = i \\ \boldsymbol{\Sigma}_{\mathcal{C}_{ik}} + \left(\Delta\tilde{\mathbf{R}}_{ik}\mathbf{f}_R(\boldsymbol{\alpha}_k)\Delta t\right)\boldsymbol{\Sigma}_{vd}\left(\Delta\tilde{\mathbf{R}}_{ik}\mathbf{f}_R(\boldsymbol{\alpha}_k)\Delta t\right)^{\top} & \text{for } k > i \end{cases} \quad (59)$$

starting with  $\boldsymbol{\Sigma}_{\mathcal{C}_{ii}} = \mathbf{0}_{3,3}$ , where  $\boldsymbol{\Sigma}_{vd}$  is the covariance of the discrete contact velocity noise  $\boldsymbol{\eta}_k^{vd}$ .

## 6 Point Contact Factor Jacobians

### 6.1 Jacobians of $\mathbf{r}_{\Delta\mathbf{d}_{ij}}$

Since we are omitting the contact frame's orientation for the preintegrated point contact factor, we adopt the following retraction  $\mathbf{d} \leftarrow \mathbf{d} + \mathbf{R}\delta\mathbf{d}$ . The retraction for the body orientation remains as in (20). The Jacobians of the point contact factor residuals can now be computed as:

$$\begin{aligned} \mathbf{r}_{\Delta\mathbf{d}_{ij}}(\mathbf{R}_i\text{Exp}(\delta\boldsymbol{\phi}_i)) &= (\mathbf{R}_i\text{Exp}(\delta\boldsymbol{\phi}_i))^{\top}(\mathbf{d}_j - \mathbf{d}_i) \\ &= \text{Exp}(-\delta\boldsymbol{\phi}_i)\mathbf{R}_i^{\top}(\mathbf{d}_j - \mathbf{d}_i) \\ &= (\mathbf{I} - \delta\boldsymbol{\phi}_i^{\wedge})\mathbf{R}_i^{\top}(\mathbf{d}_j - \mathbf{d}_i) \\ &= \mathbf{R}_i^{\top}(\mathbf{d}_j - \mathbf{d}_i) - \delta\boldsymbol{\phi}_i^{\wedge}\mathbf{R}_i^{\top}(\mathbf{d}_j - \mathbf{d}_i) \\ &= \mathbf{R}_i^{\top}(\mathbf{d}_j - \mathbf{d}_i) + (\mathbf{R}_i^{\top}(\mathbf{d}_j - \mathbf{d}_i))^{\wedge}\delta\boldsymbol{\phi}_i \\ &= \mathbf{r}_{\Delta\mathbf{d}_{ij}}(\mathbf{R}_i) + (\mathbf{R}_i^{\top}(\mathbf{d}_j - \mathbf{d}_i))^{\wedge}\delta\boldsymbol{\phi}_i \end{aligned} \quad (60)$$

$$\begin{aligned} \mathbf{r}_{\Delta\mathbf{d}_{ij}}(\mathbf{d}_i + \mathbf{R}_i\delta\mathbf{d}_i) &= \mathbf{R}_i^{\top}(\mathbf{d}_j - (\mathbf{d}_i + \mathbf{R}_i\delta\mathbf{d}_i)) \\ &= \mathbf{R}_i^{\top}(\mathbf{d}_j - \mathbf{d}_i - \mathbf{R}_i\delta\mathbf{d}_i) \\ &= \mathbf{R}_i^{\top}(\mathbf{d}_j - \mathbf{d}_i) - \mathbf{R}_i^{\top}\mathbf{R}_i\delta\mathbf{d}_i \\ &= \mathbf{r}_{\Delta\mathbf{d}_{ij}}(\mathbf{d}_i) - \delta\mathbf{d}_i \end{aligned} \quad (61)$$

$$\begin{aligned}
\mathbf{r}_{\Delta \mathbf{d}_{ij}}(\mathbf{d}_j + \mathbf{R}_j \delta \mathbf{d}_j) &= \mathbf{R}_i^\top ((\mathbf{d}_j + \mathbf{R}_j \delta \mathbf{d}_j) - \mathbf{d}_i) \\
&= \mathbf{R}_i^\top (\mathbf{d}_j + \mathbf{R}_j \delta \mathbf{d}_j - \mathbf{d}_i) \\
&= \mathbf{R}_i^\top (\mathbf{d}_j - \mathbf{d}_i) + \mathbf{R}_i^\top \mathbf{R}_j \delta \mathbf{d}_j \\
&= \mathbf{r}_{\Delta \mathbf{d}_{ij}}(\mathbf{d}_j) + \mathbf{R}_i^\top \mathbf{R}_j \delta \mathbf{d}_j
\end{aligned} \tag{62}$$

Written concisely, the Jacobians of  $\mathbf{r}_{\Delta \mathbf{d}_{ij}}$  are,

$$\begin{aligned}
\frac{\partial \mathbf{r}_{\Delta \mathbf{d}_{ij}}}{\partial \delta \phi_i} &= \left( \mathbf{R}_i^\top (\mathbf{d}_j - \mathbf{d}_i) \right)^\wedge \\
\frac{\partial \mathbf{r}_{\Delta \mathbf{d}_{ij}}}{\partial \delta \mathbf{p}_i} &= \mathbf{0}_{3,3} \\
\frac{\partial \mathbf{r}_{\Delta \mathbf{d}_{ij}}}{\partial \delta \theta_i} &= \mathbf{0}_{3,3} \\
\frac{\partial \mathbf{r}_{\Delta \mathbf{d}_{ij}}}{\partial \delta \mathbf{d}_i} &= -\mathbf{I}_3 \\
\frac{\partial \mathbf{r}_{\Delta \mathbf{d}_{ij}}}{\partial \delta \phi_j} &= \mathbf{0}_{3,3} \\
\frac{\partial \mathbf{r}_{\Delta \mathbf{d}_{ij}}}{\partial \delta \mathbf{p}_j} &= \mathbf{0}_{3,3} \\
\frac{\partial \mathbf{r}_{\Delta \mathbf{d}_{ij}}}{\partial \delta \theta_j} &= \mathbf{0}_{3,3} \\
\frac{\partial \mathbf{r}_{\Delta \mathbf{d}_{ij}}}{\partial \delta \mathbf{d}_j} &= \mathbf{R}_i^\top \mathbf{R}_j
\end{aligned} \tag{63}$$

## References

- [1] R. Hartley, J. Mangelson, L. Gan, M. Ghaffari Jadidi, J. M. Walls, R. M. Eustice, and J. W. Grizzle, “Legged robot state-estimation through combined kinematic and preintegrated contact factors,” in *Proc. IEEE Int. Conf. Robot. Automat.*, 2018.
- [2] C. Forster, L. Carlone, F. Dellaert, and D. Scaramuzza, “On-manifold preintegration for real-time visual-inertial odometry,” *IEEE Trans. Robot.*, vol. 33, no. 1, pp. 1–21, 2017.
